# Supplementary material for: Conservation of Fractional Mean Energy in Dissipative Gases
Source: arXiv:2210.06193 source file (2022-10-11)
Supplement: Supplementary file 1 [file main_supplemental.tex]

\documentclass[%
 reprint,
%superscriptaddress,
%groupedaddress,
%unsortedaddress,
%runinaddress,
%frontmatterverbose,
%preprint,
%preprintnumbers,
%nofootinbib,
%nobibnotes,
%bibnotes,
 amsmath,amssymb,
 aps,
%pra,
%prb,
%rmp,
%prstab,
%prstper,
%floatfix,
]{revtex4-1}

\usepackage{graphicx}% Include figure files

\begin{document}
\input{supplemental.tex}

\bibliography{../refs} % Produces the bibliography via BibTeX.
\end{document}
